# Supplementary material for: MeshAvatar: Learning High-quality Triangular Human Avatars from Multi-view Videos
Source: arXiv:2407.08414 source file (2024-07-11)
Supplement: Supplementary file 1 [file appendix.tex]

\begin{figure*}
    \centering
    \includegraphics[width=\linewidth]{figures/rec.pdf}
    \caption{\textbf{More reconstruction results}, including reconstructed geometry, albedo color, material roughness, and light probes. }
    \label{fig:rec-more}
\end{figure*}

\begin{figure*}
    \centering
    \includegraphics[width=\linewidth]{figures/animate.pdf}
    \caption{\textbf{More animation results} given the novel poses from AMASS dataset~\cite{mahmood2019amass} and novel lighting conditions. }
    \label{fig:animte-more}
\end{figure*}

\begin{figure*}[t]
\begin{minipage}{0.48\linewidth}
    \centering
    \includegraphics[width=\linewidth]{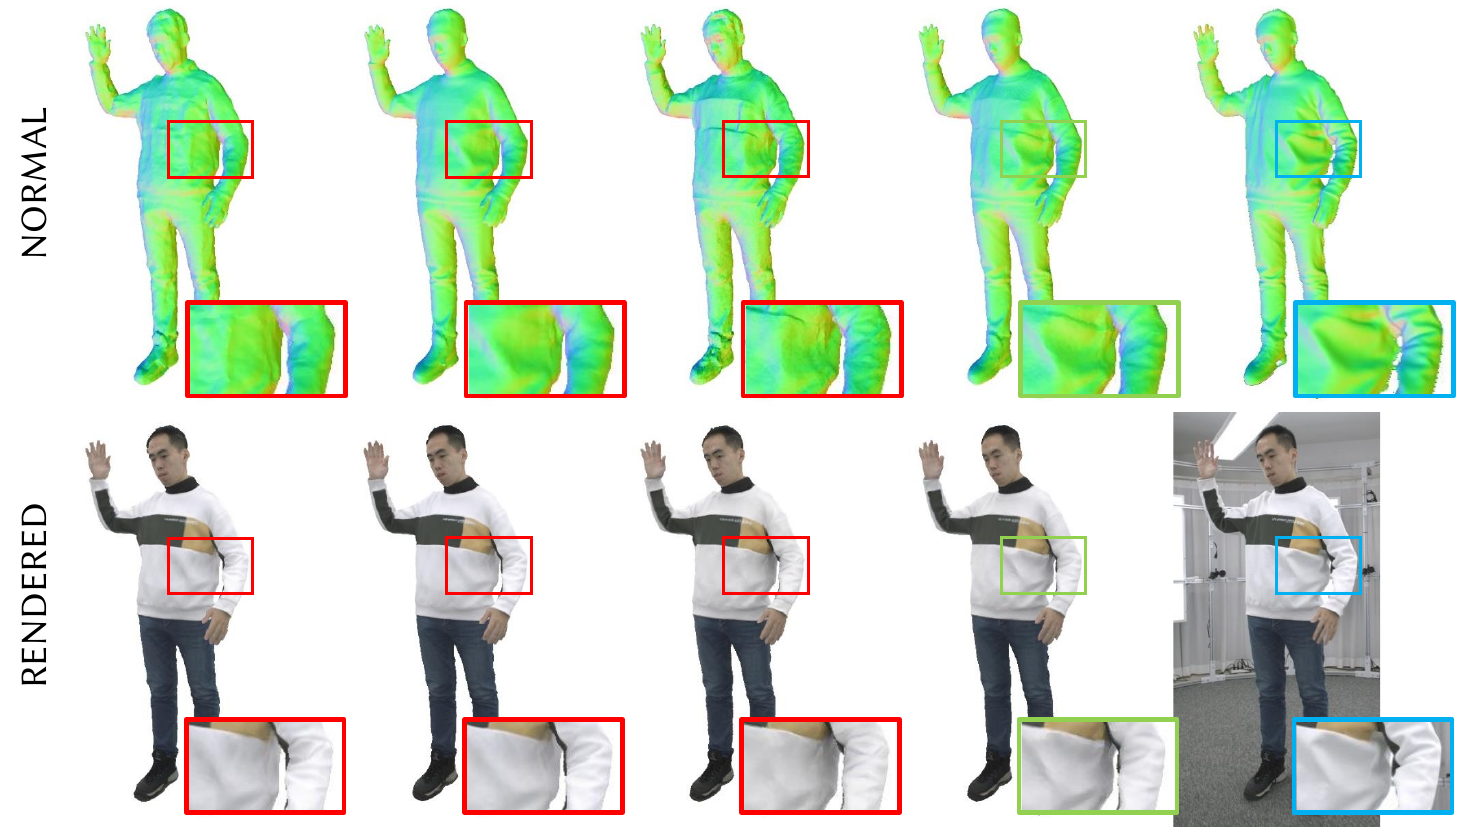}
    \caption{\textbf{Ablation Study.} (a) w/o PBR and normal; (b) w/o PBR; (c) w/o normal; (d) ours; (e) reference image and estimated normal. }
    \label{fig:ablation}
\end{minipage}
\hfill
\begin{minipage}{0.48\linewidth}
    \centering
    \includegraphics[width=\linewidth]{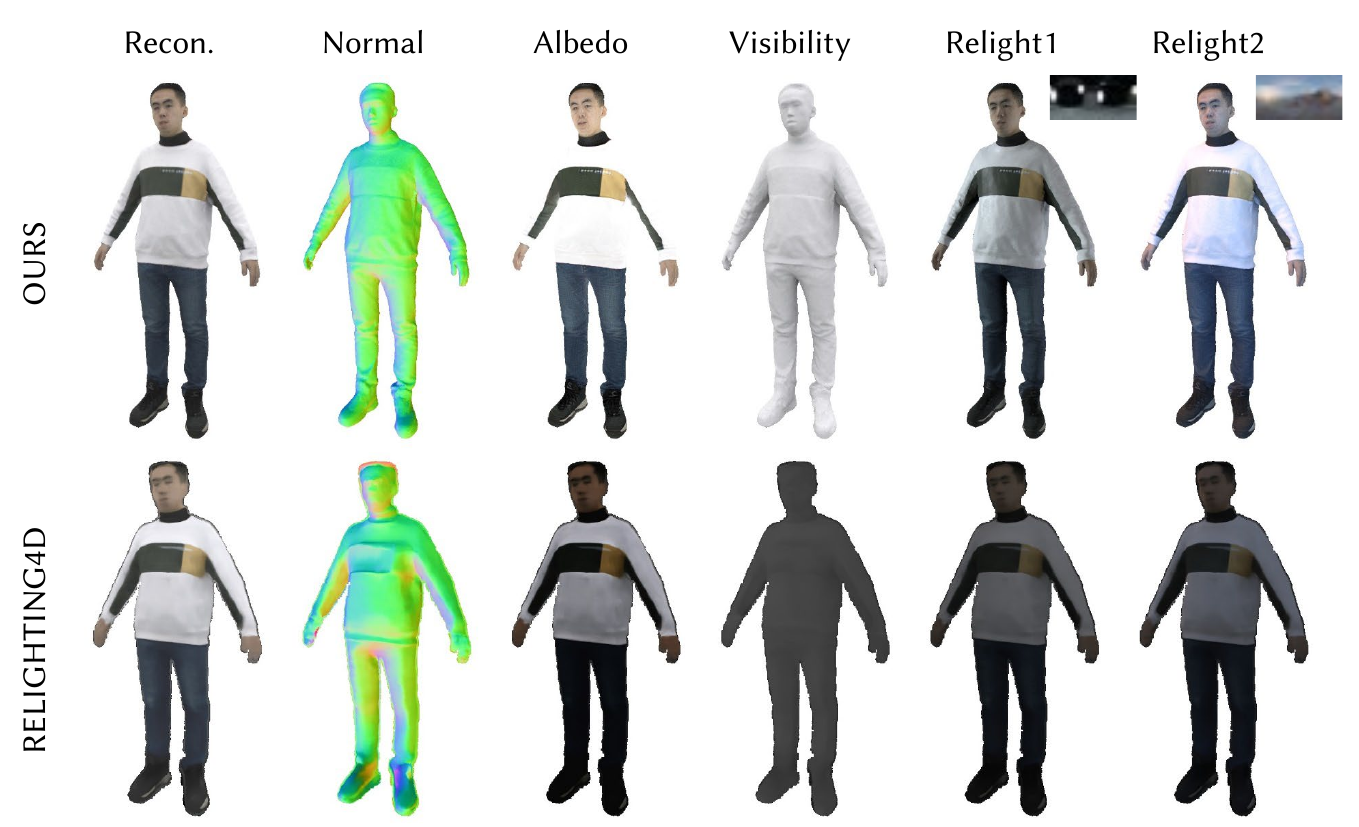}
    \caption{\textbf{Relighting comparison} against Relighting4D~\cite{chen2022relighting4d}. }
    \label{fig:relight}
\end{minipage}
\end{figure*}
